# Supplementary material for: Combining Offline Causal Inference and Online Bandit Learning for Data Driven Decision
Source: arXiv:2001.05699 source file (2020-11-07)
Supplement: Supplementary file 1 [file supplement.tex]

The latex source of this PDF file can be found in the ``ICML2020\_supplement''
folder in the ``latexsource.zip''.
This supplementary materials include three parts: (1) more algorithmic
instances using our framework; (2) supplementary experimental results and detailed
experiment settings; (3) an appendix that contains the proofs of all the theorems.

Before we start, we want to show a snippet of our experiment results. The
following Figure~\ref{fig:yahoo_linUCB_forest} show experiment results on Yahoo's
 news recommendation dataset, where the left figure is for the {\em
  LinUCB} algorithm and the right figure is for the {\em $\epsilon$-greedy
  causal forest} algorithm. We see that these two algorithms have comparable
cummulative reward after 3500 rounds. We note that the Yahoo's news
recommendation dataset is generated via a bilinear model so that the
contexts and a reward follow a linear relationship~\cite{chu2009case}. In this case,
the linear model and LinUCB correctly model the data. Even in this case, we can
see our non-parametric {\em $\epsilon$-greedy causal forest} can achieve
comparable performances.

\begin{figure}[htb]
  \begin{minipage}{1.05\linewidth}
    \includegraphics[width=0.49\textwidth]{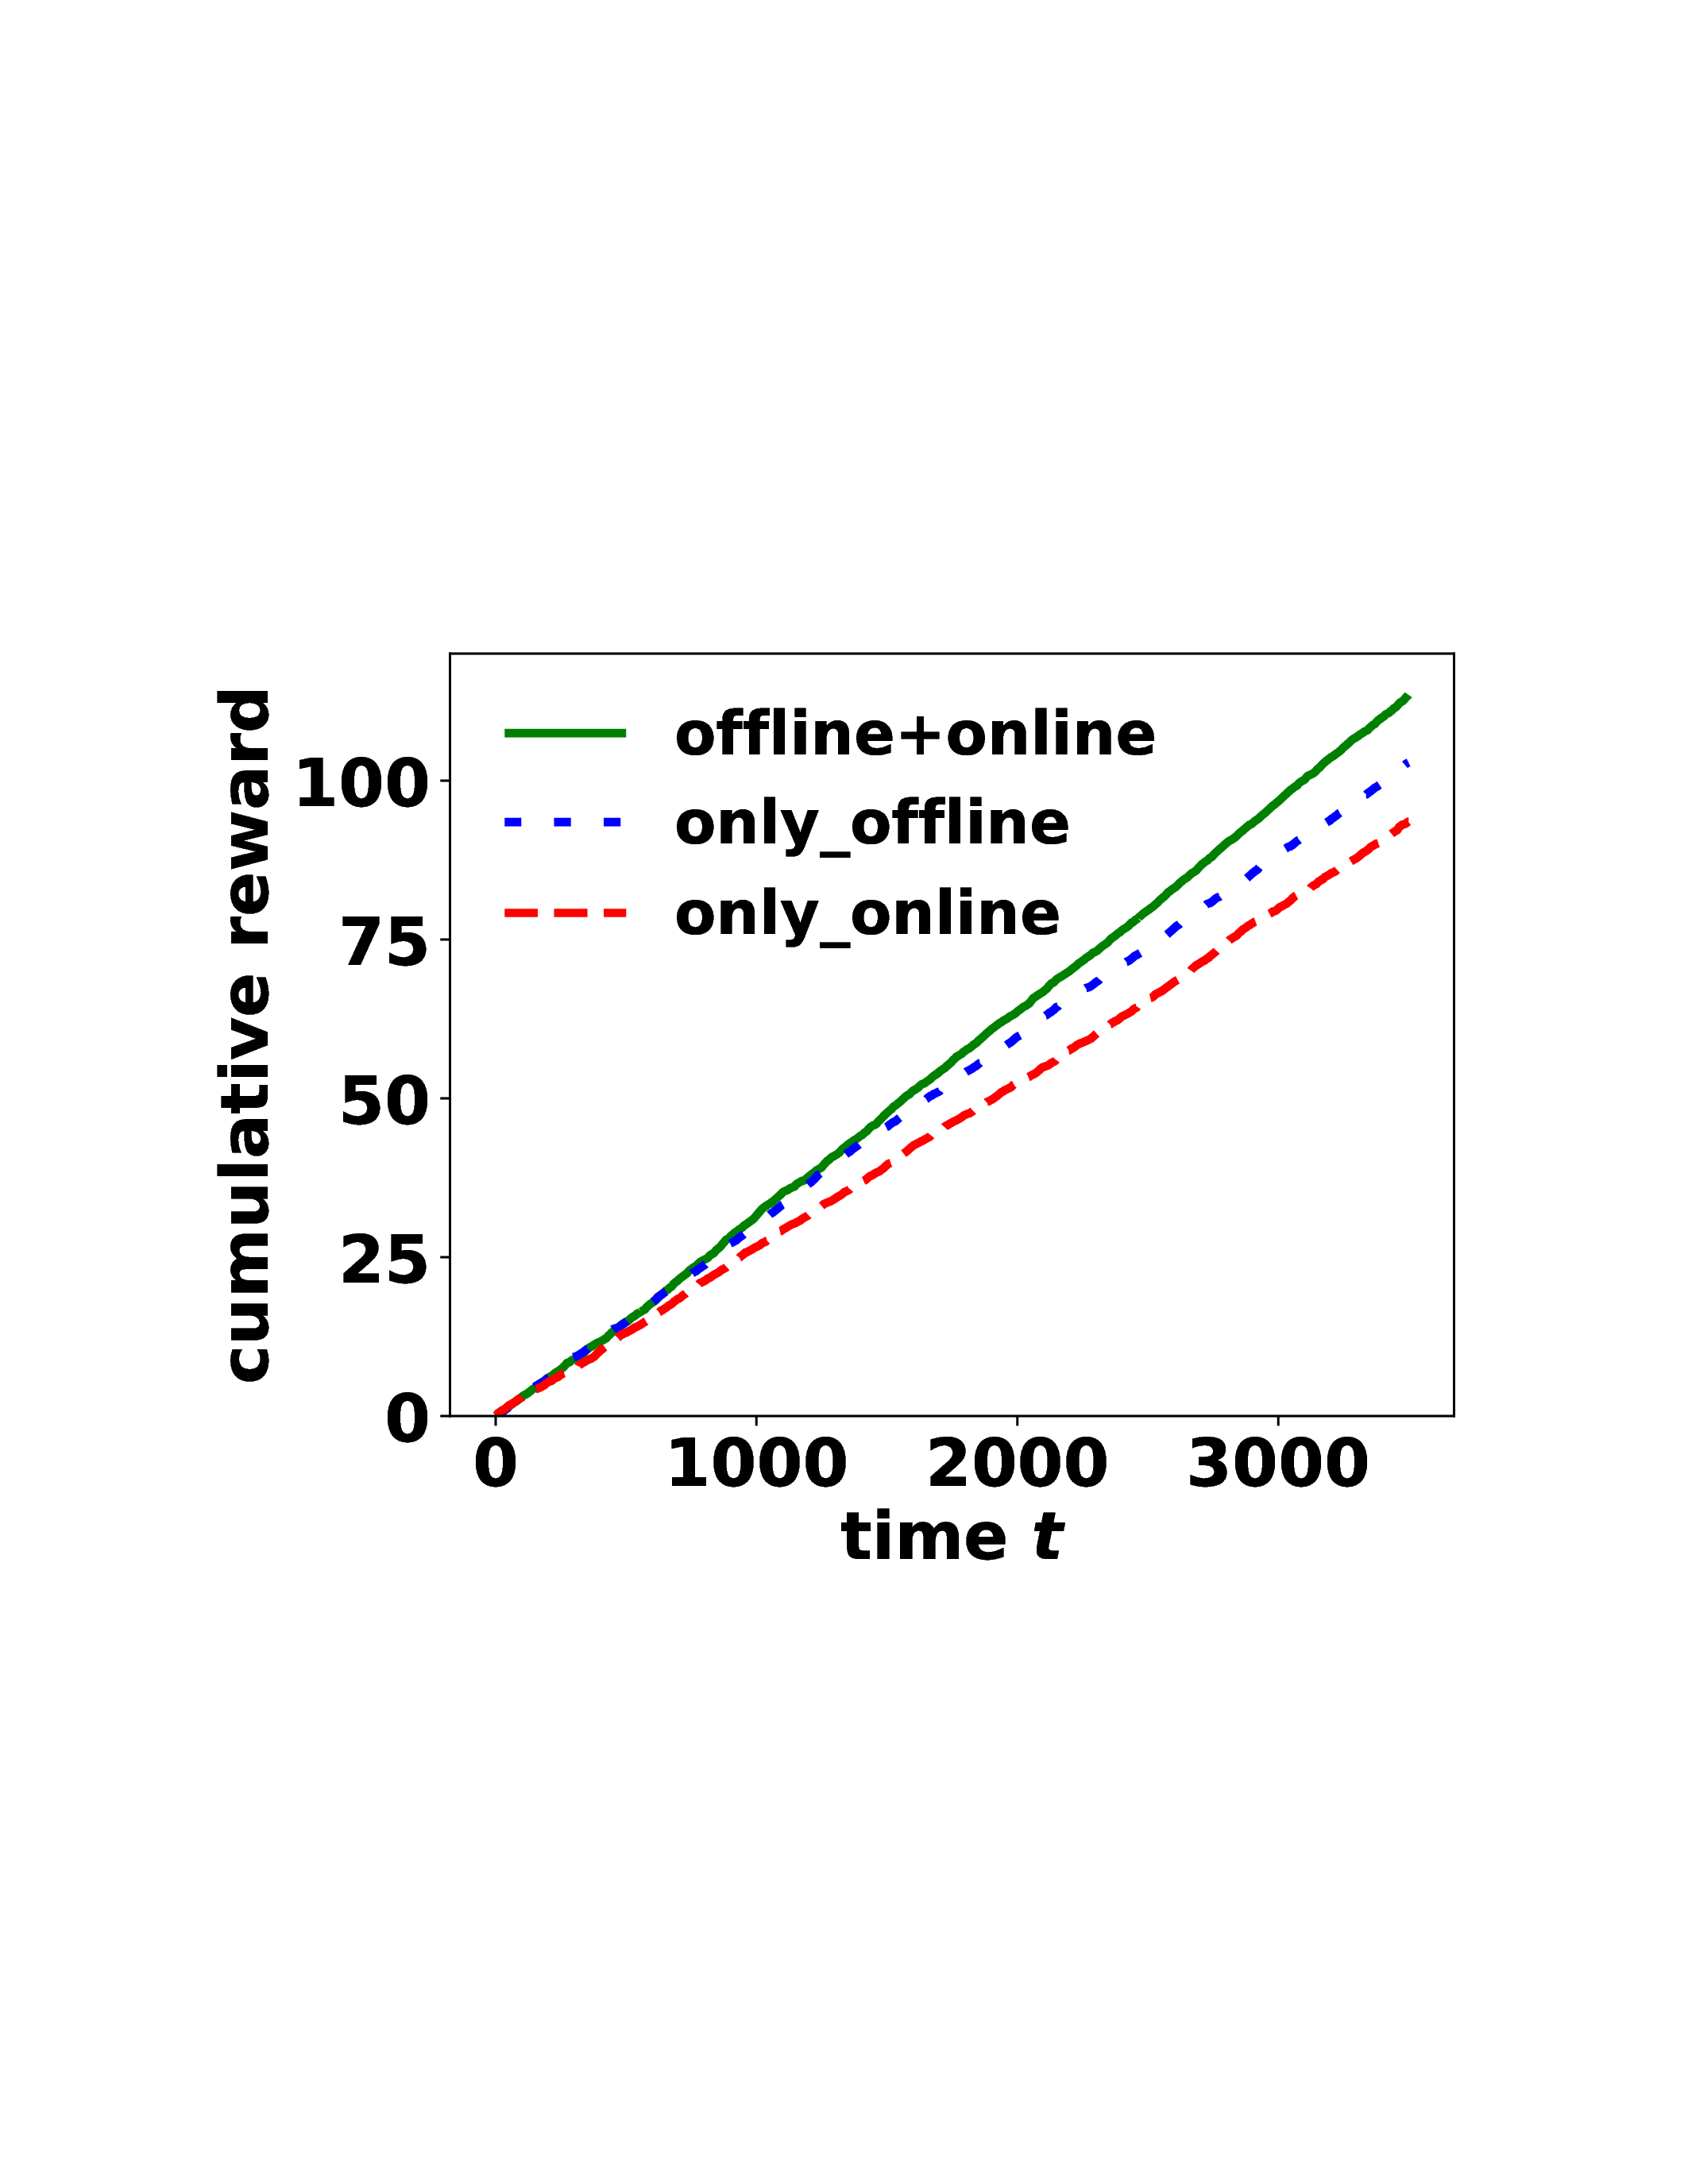}
    \includegraphics[width=0.49\textwidth]{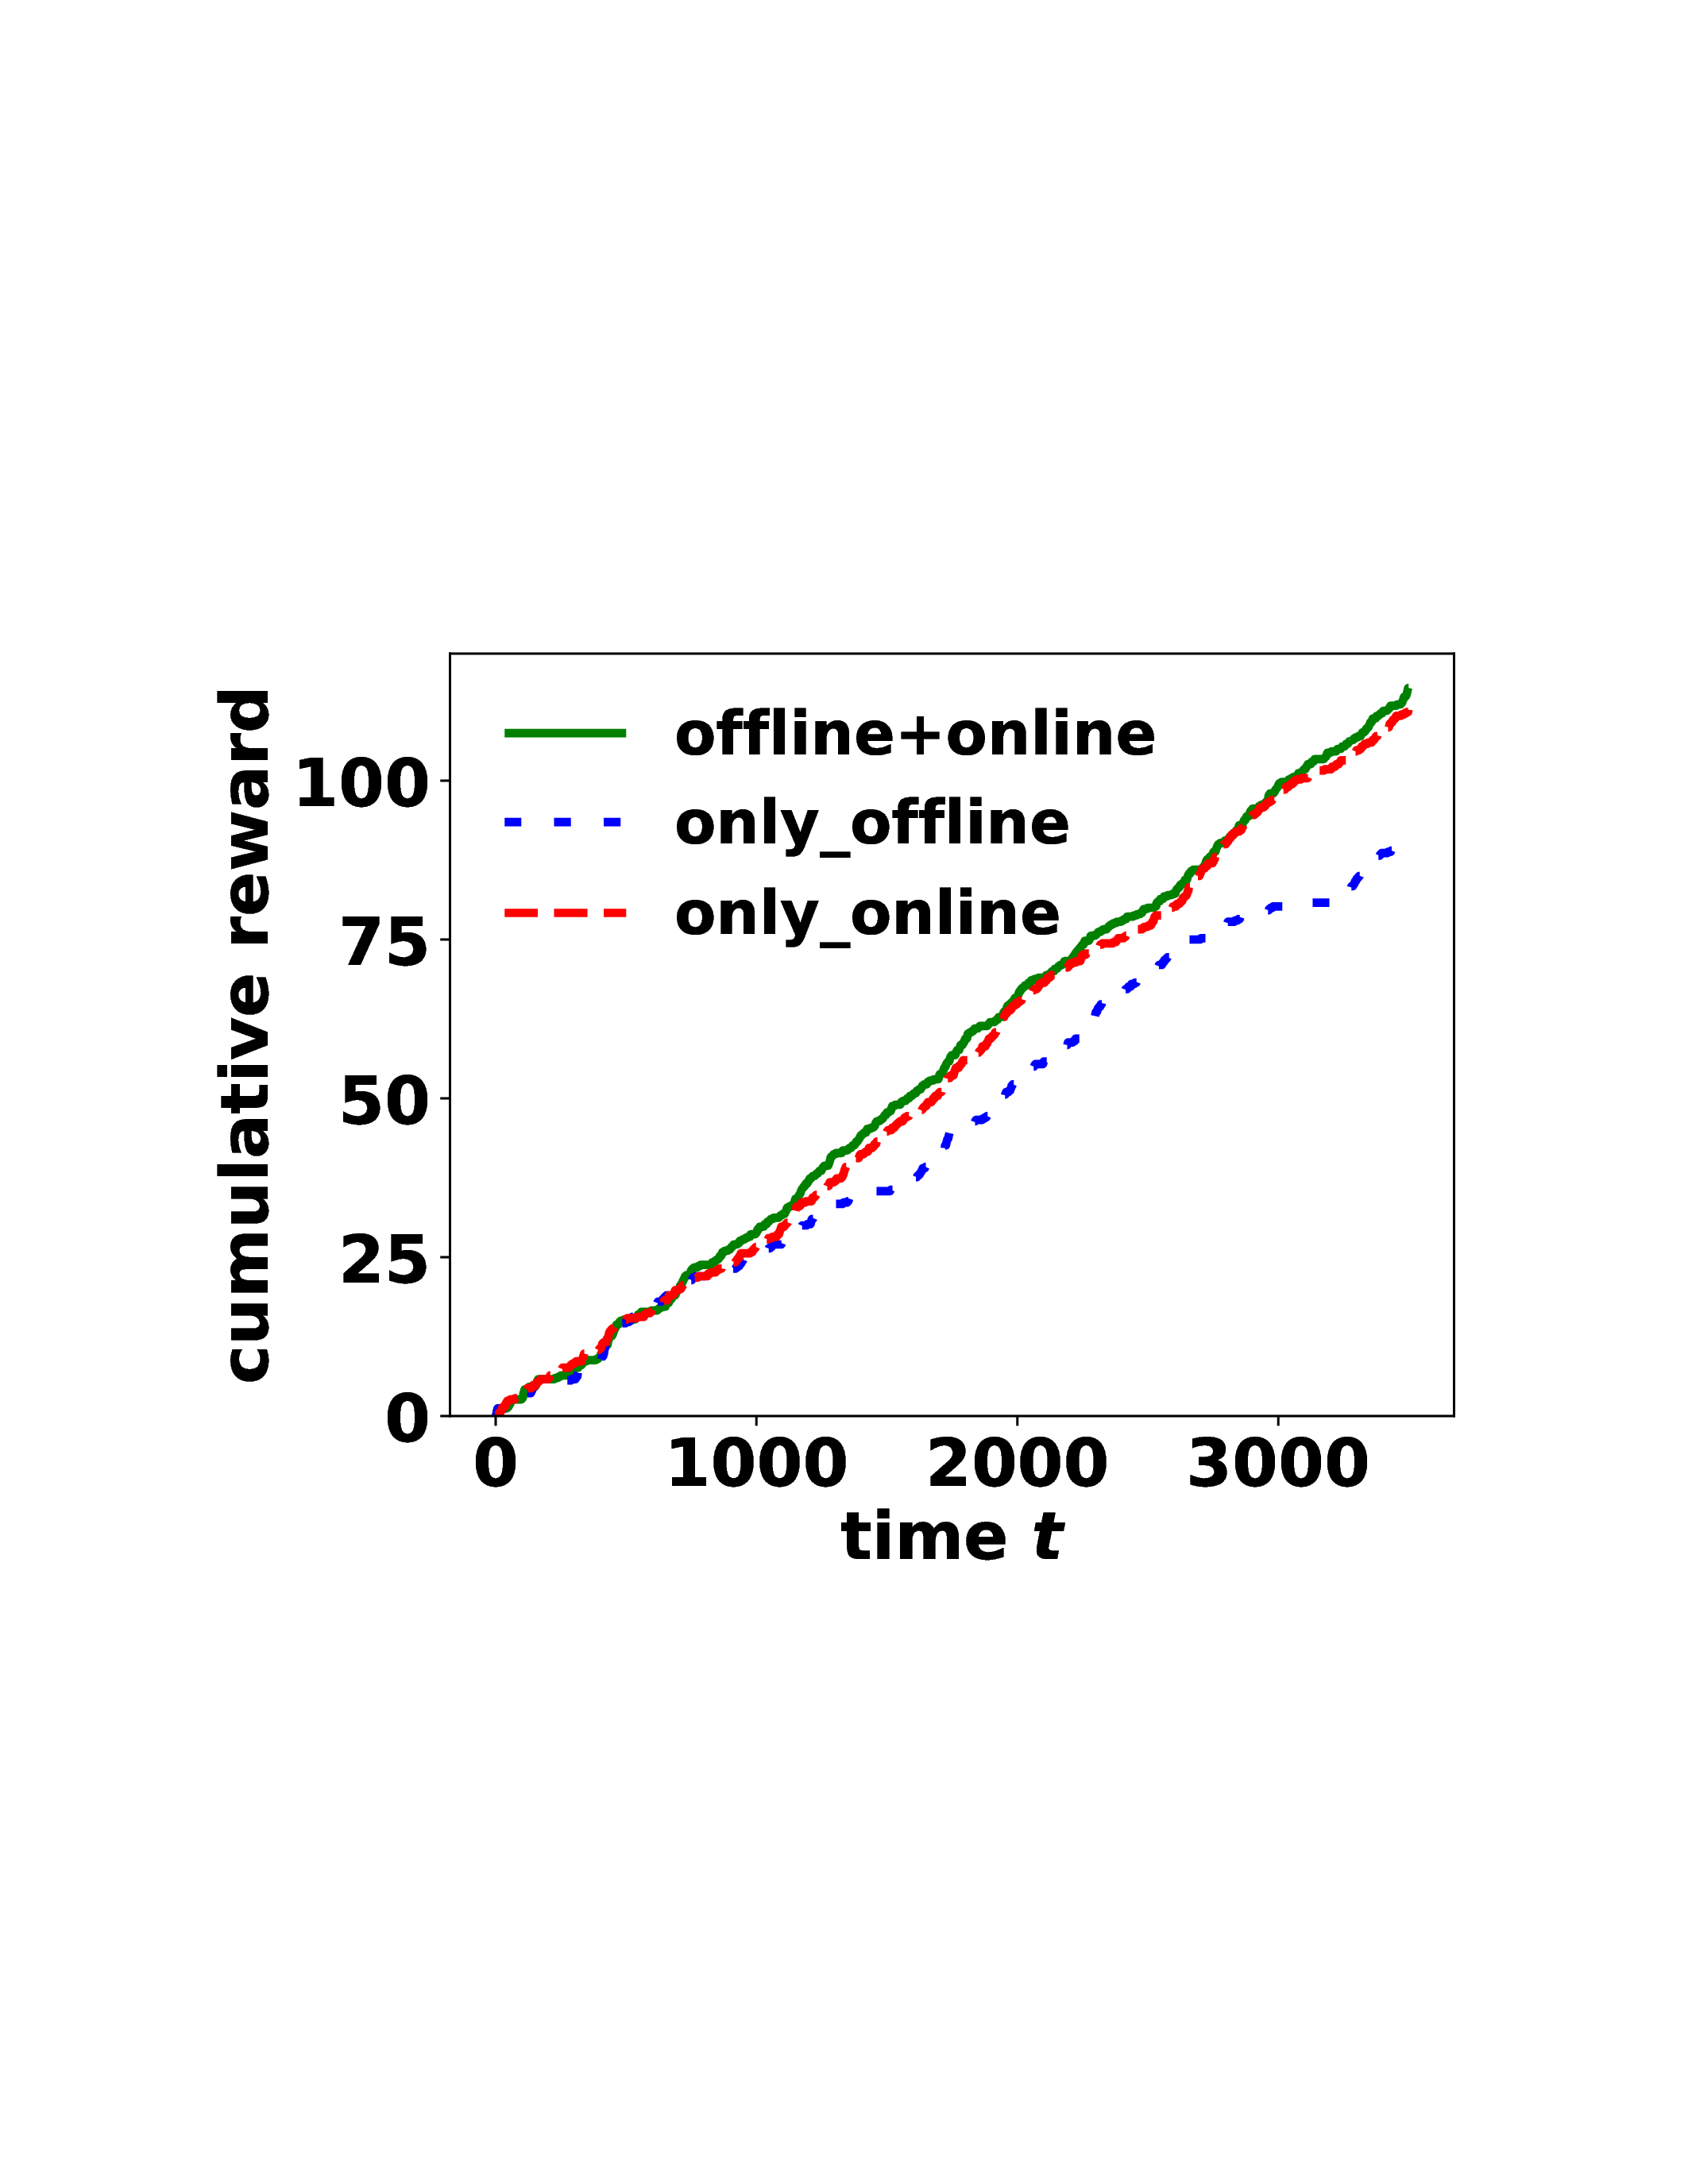}
    \caption{The left figure is the result of the {\em LinUCB} algorithm and its
      variants (average of 50 runs). The right figure is the
      result of the {\em $\epsilon$-greedy causal forest} (average of 5 runs).}
  \label{fig:yahoo_linUCB_forest}
  \end{minipage}
\end{figure}

We also run the ``PS matching + UCB'' and ``PS weighting + UCB'' using the Yahoo
news recommenation dataset. Although the Yahoo data originally evalues the
contextual bandit algorithms, we can use it to .

For the ``PS matching + UCB'' algorithm in Figure~\ref{fig:ps_matching_yahoo}, we use 1,000 offline data samples, and
repeat for 1,000 times to take the average.

\begin{figure}[htb]
  \begin{minipage}{0.5\linewidth}
    \includegraphics[width=\textwidth]{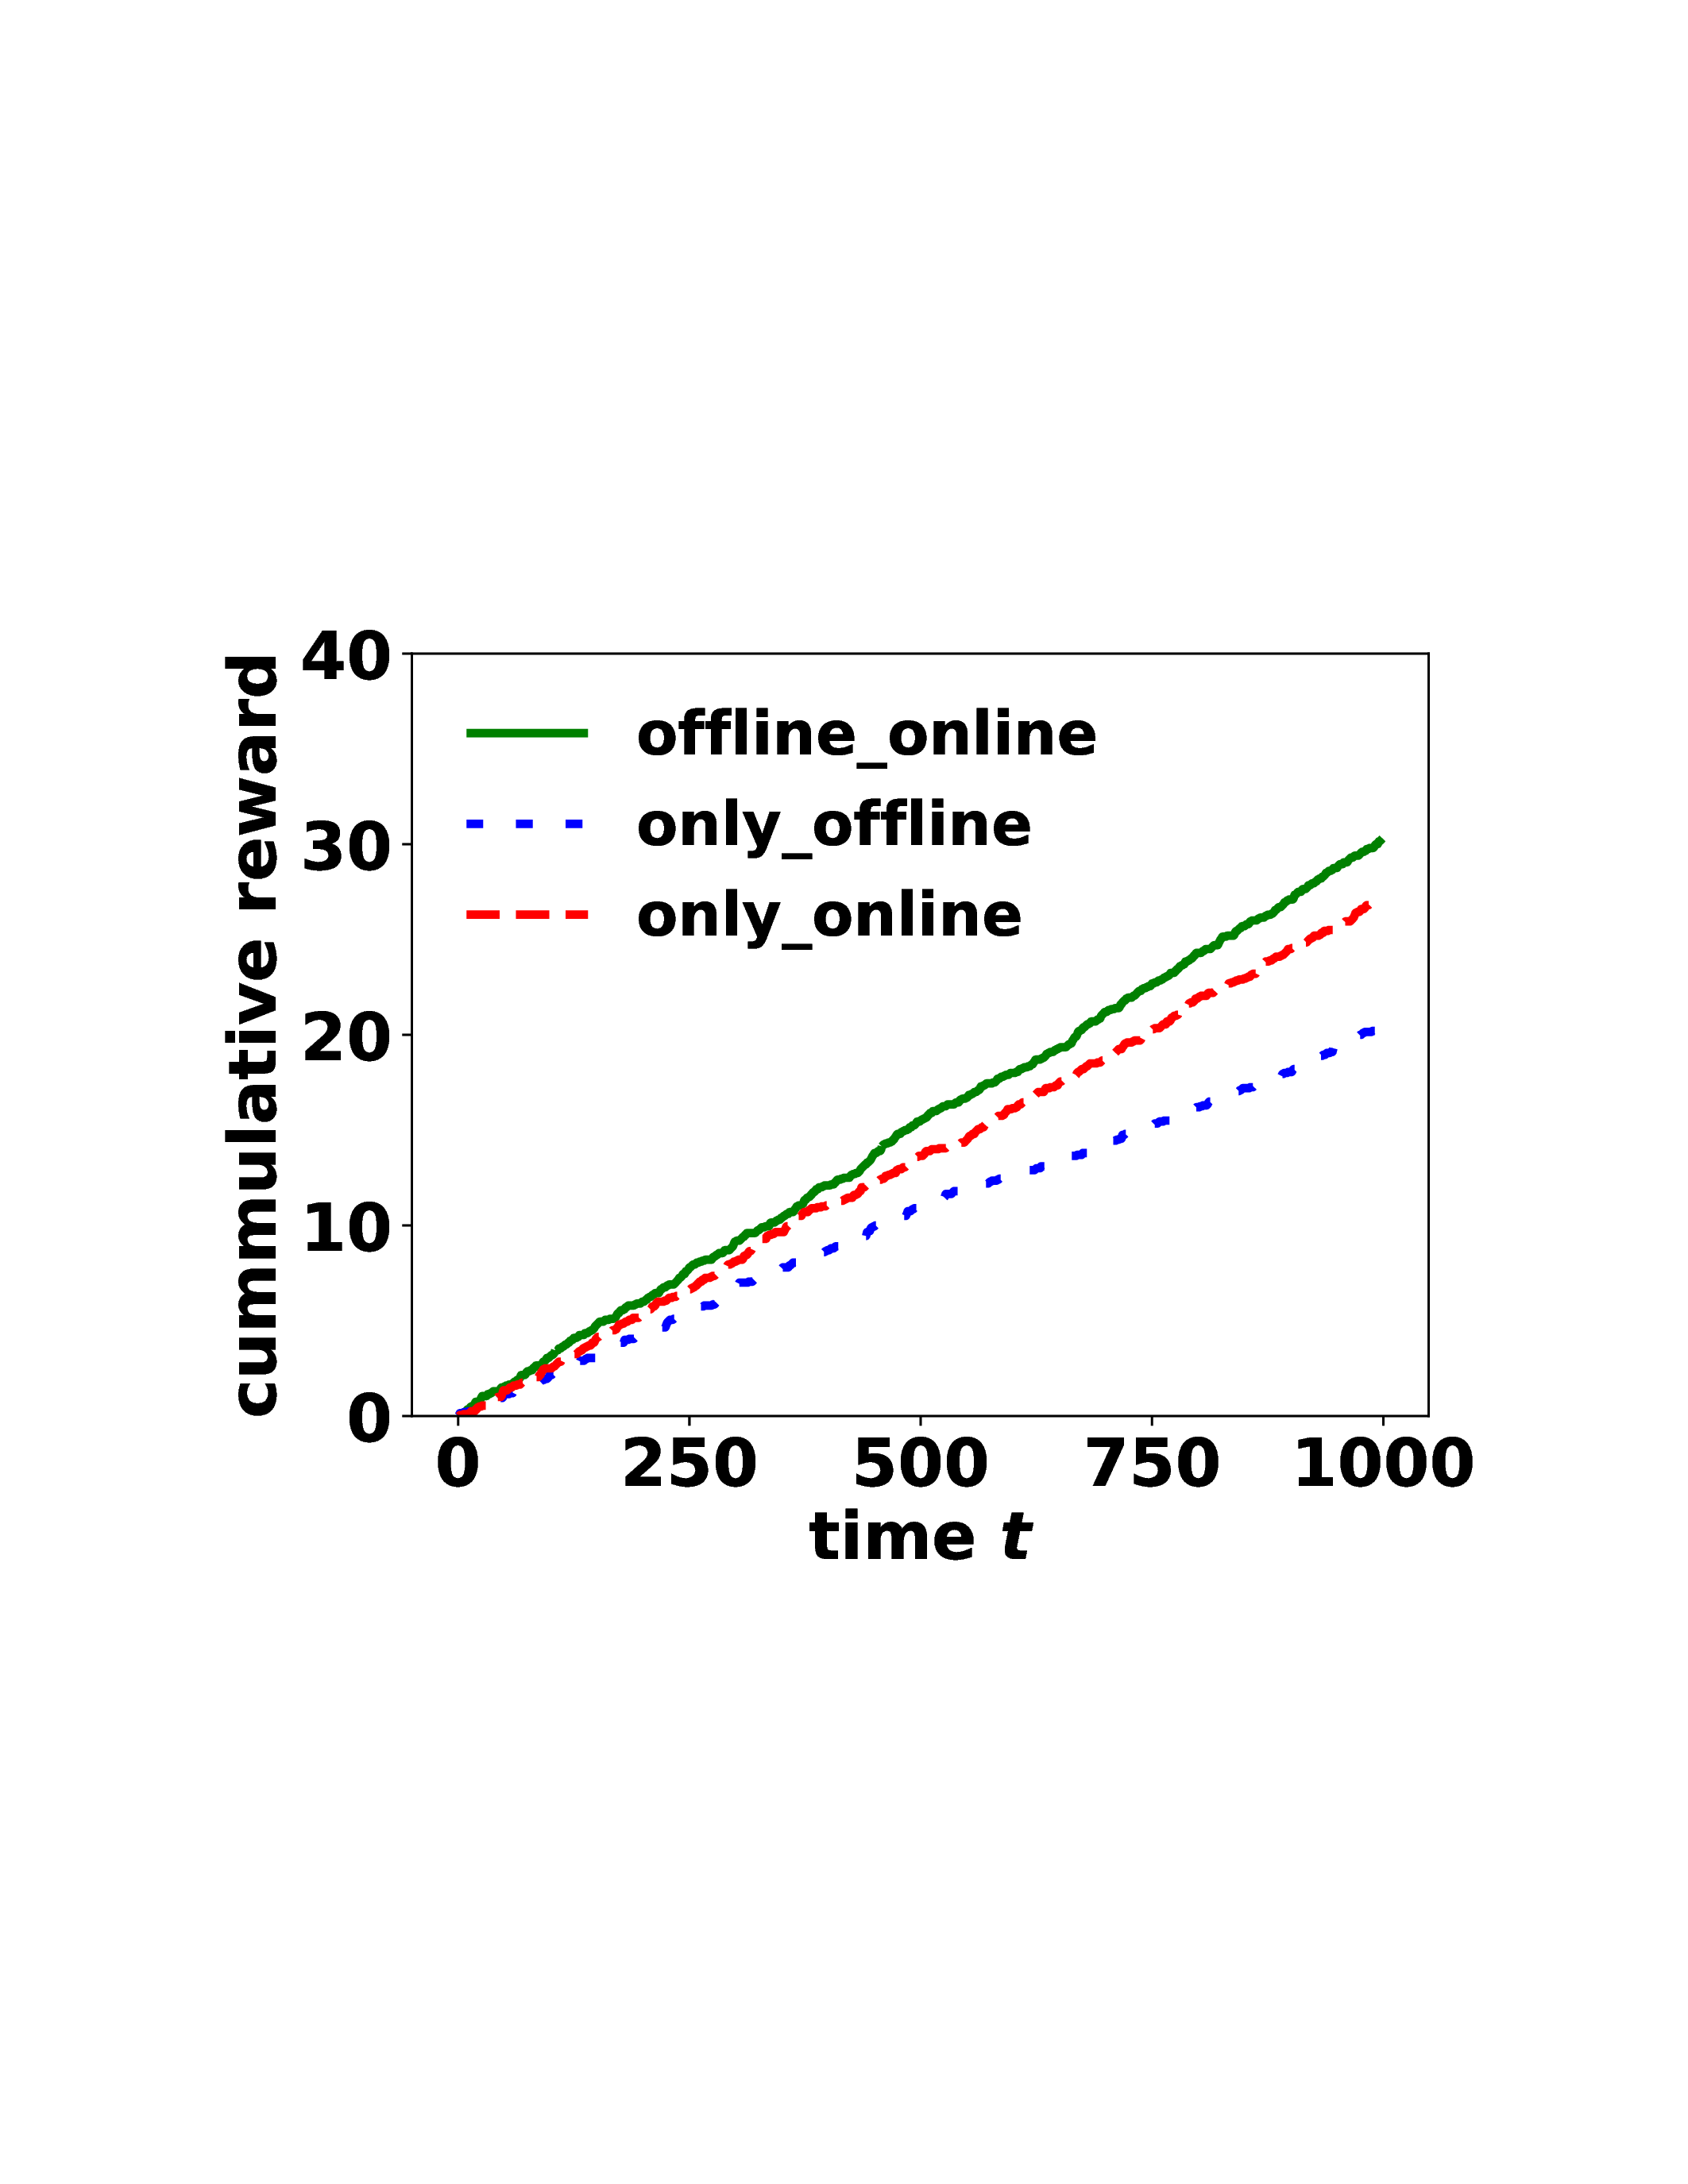}
    \caption{PS matching + UCB ($\CA_1$) on the Yahoo dataset}
    \label{fig:ps_matching_yahoo}
  \end{minipage}
\end{figure}

\vspace{0.1in}
\noindent{\bf \LARGE Part 1: More Algorithms and More Regret Analysis}
% \vspace{-0.1in}

In this part, we present the supplementary algorithmic instances that cannot be
covered in the main paper due to the page limits. The section names in this part
correspond to the section names in the main paper. In
Section~\ref{sec:sup_framework}, we introduce the A/B test online bandit oracle
and use this orcle to show that causal inference is a special case of our framework.
In Section~\ref{sec:sup_context_independent}, we introduce two instances of
algorithms for context-independent decisions. In
Section~\ref{sec:sup_contextual}, we show how we combine linear regression and
the LinUCB algorithm to make contextual decisions. For the above algorithmic
instances, we provide the regret upper bounds.

\section{General Algorithmic Framework}
\label{sec:sup_framework}

\makeatletter
\renewcommand{\ALG@name}{Instance}
\makeatother

\subsection{Algorithmic Framework}

% for supplement to use
% \begin{comment}
\noindent{\bf Unifying causal inference and online bandit learning.}
Both online bandit algorithms and causal inference
algorithms are special cases of our framework.
First, if there are no logged data, then the offline evaluator cannot synthesize
feedbacks and will always return {``NULL''}.  
In this case, our framework always calls the online bandit oracle, and
reduces to an online bandit algorithm.
Second, let's consider the A/B test online learning oracle in
Instance~\ref{alg:abtest_oracle} and the case $T{=}1$.  
Then, after the offline phase, the estimated outcome $\bar{y}_a$ for action $a$ estimates the causal effect. 
In this case, our framework reduces to a causal inference algorithm.

\setcounter{algorithm}{5}

% \vspace{-0.1in}
\begin{algorithm}
  % \SetAlgorithmName{Class}{class}{List of Classes}
  \caption{\bf {\small (Online Bandit Oracle)} - A/B test}\label{alg:abtest_oracle}
  \begin{algorithmic}[1]
  \STATE {\bf Variables:} average outcome $\bar{y}_a$ of each action 
 $a{\in}[K]$, and the number of times $n_a$ that action $a$ was played.
  % \SetKwFunction{FPlay}{{\bf play}}
  \FUNCTION{{\it play}($\bm{x}$)}
    \STATE \textbf{return} $a$ with probability $1/K$ for each $a\in[K]$
  \ENDFUNCTION
  % \SetKwFunction{FUpdate}{{\bf update}}
  \FUNCTION{{\it update}($\bm{x}, a, y$)}
    \STATE \textbf{return} $\bar{y}_a \gets n_a\bar{y}_a / (n_a+1)$,~~~~  $n_a \gets n_a + 1$ 
  \ENDFUNCTION
  \end{algorithmic}
\end{algorithm}
% \vspace{-0.15in}
% \end{comment}

\subsection{Regret Analysis Framework}

% for supplement uses
\begin{manualtheorem}{5}[General lower bound]
  \label{mthm:general_lower_bound}
  Suppose for any bandit oracle $\widetilde{\CO}$, $\exists$ a
  non-decreasing function
  $h(T)$, s.t. $R(T, \widetilde{\CO}){\ge} h(T)$ for $\forall T$.
 % where $h(T)$ is the regret lower bound for all possible algorithms.
 The offline
  estimator returns unbiased outcomes $\{\tilde{y}_j\}_{j=1}^N$ w.r.t. $\{(\tilde{\bm{x}}_j,\tilde{a}_j)\}_{j=1}^N$. Then for any
  contextual-independent algorithm $\widetilde{\CA}$ we have:
 \vspace{-0.1in}
 \begin{align*}
  R(T, \widetilde{\CA}) \ge h(T) - \sum\nolimits_{j=1}^N\left( \max_{a\in[K]}\MBE[y|a] - \MBE[y|a=\tilde{a}_j] \right).
 \vspace{-0.1in}
 \end{align*}
 For any contextual algorithm $\widetilde{\CA}_c$, we have
 \vspace{-0.1in}
 \begin{align*}
   R(T, \widetilde{\CA}_c) {\ge} h(T) {-} \hspace{-0.05in}\sum\nolimits_{j=1}^N \hspace{-0.05in}
   \left( \max_{a\in[K]}\MBE[y|a,\tilde{\bm{x}}_j] {-} \MBE[y|a{=}\tilde{a}_j{,} \tilde{\bm{x}}_j] \right).
 \vspace{-0.1in}
 \end{align*}
 %  \label{thm:general_lower_bound}
 %  Suppose for any online bandit oracle $\widetilde{\CO}$, there exists a function
 %  $h(T)$, such that $R(T, \widetilde{\CO})\ge h(T)$ for $\forall T$. Then for any
 %  contextual-independent algorithm $\widetilde{\CA}$ we have:
 % \begin{align*}
 %  R(T, \widetilde{\CA}) \ge h(T+N) - \sum\nolimits_{i=1}^I\left( \max_{a\in[K]}\MBE[y|a] - \MBE[y|a=a_i] \right).
 % \end{align*}
 % We also have a regret bound for any contextual algorithm $\widetilde{\CA}_c$:
 % \begin{align*}
 %   R(T, \widetilde{\CA}_c) \ge h(T+N) - \sum\nolimits_{i=1}^I \hspace{-0.04in}
 %   \left( \max_{a\in[K]}\MBE[y|a,\bm{x}_i] - \MBE[y|a=a_i, \bm{x}_i] \right).
 % \end{align*}
\vspace{-0.1in}
\end{manualtheorem}
\begin{proof}
 All proofs are in the appendix of the Part 3.
\end{proof}
\vspace{-0.1in}
\noindent Theorem~\ref{mthm:general_lower_bound} shows how we can apply the regret lower
bound of online bandit oracles~\cite{bubeck2013bounded} to derive a regret lower
bound with logged data . 
When an algorithm's upper bound meets the lower bound, we get a {\em nearly optimal}
algorithm for online decision making with logged data.
% In fact, if $\lim_{T\rightarrow T}
% h(T)/g(T){>}0$, and all the logged samples are used, then the algorithm $\CA$
% achieves the optimal regret.

\section{Case Study: Context-independent Decision}
\label{sec:sup_context_independent}
% \begin{comment}
\subsection{A Warm Up Case - Exact Matching + UCB ($\CA_0$)} 

{\bf Algorithm description. }
Let us start with the instance $\CA_0$ that applies Algorithm~1 
to speed up the UCB algorithm with ``exact matching'' (i.e., a simple method in causal inference).  
% The online bandit oracle Upper Confidence Bound (UCB)~\cite{auer2002finite} is described as an objective-oriented Class~\ref{alg:ucb}.  
In each decision round, the oracle selects an action with the maximum 
upper confidence bound defined as 
$\bar{y}_a{+}\beta\sqrt{{2\ln(n)}/{n_a}}$, 
where 
$\bar{y}_a$ is the average outcome, 
$\beta$ is a constant, and $n_a$ is the
number of times that an action $a$ was played (Line 1).

  % \vspace{-0.1in}

Furthermore, we instantiate the offline evaluator with 
the ``exact matching''\cite{stuart2010matching} method outlined in Instance~\ref{alg:exact_match}.   
It searches for a data item in log $\CL$ with the exact same context $\bm{x}$ and action
$a$, and returns the outcome of that data item.  
If it cannot find a matched data item for an action $a$, then it stops the
subsequent matching process for the action $a$.  
The stop of matching is to ensure
that the synthetic feedbacks simulate the online feedbacks correctly.   

% \vspace{-0.1in}
\begin{algorithm}
  % \SetAlgorithmName{Class}{class}{List of Classes}
  \caption{\bf {\small (Offline Evaluator)} - Exact Matching}\label{alg:exact_match}
  \begin{algorithmic}[1]
  % \SetKwFunction{FExactMatching}{{\bf get\_outcome}}
  \STATE {\bf Member variables}: $S_a{\in}\{False,True\}$ indicates whether we stop matching
for action $a$, initially $S_a{\gets} False, \forall a{\in}[K]$.
  \FUNCTION{exactMatching($\bm{x}$, $a$)}
    \IF{$S_a=False$}
      \STATE $\CI(\bm{x}, a)\gets \{i~|~\bm{x}_i=\bm{x}, a_i=a\}$
      \IF{$\CI(\bm{x}, a) \ne \emptyset$}
        \STATE $i\gets$ a random sample from $\CI(\bm{x},a)$
        \STATE $\CL\gets \CL \backslash \{(a_i,\bm{x}_i,y_i)\}$
        \STATE \textbf{return} $y_i$
      \ENDIF
      % \Else{
      % }
    \ENDIF
    % \Else{
      \STATE $S_a\gets True$
      \STATE \textbf{return} NULL
    % }
    % search the offline sample, to find a sample $i$ with context $\bm{x}_i=\bm{x}$ and action
    % $a_i=a$, then return the outcome $y_i$ of that sample.
    % delete this sample
    % when there is no matched outcome for $a$, always return NULL for $a$.
  \ENDFUNCTION
  \end{algorithmic}
\end{algorithm}
% \vspace{-0.2in}

% \noindent
% {\bf Regret analysis. }  
% Let  $\mathcal{A}_1$ denote the above resulting algorithm 
% that instantiate Algorithm \ref{alg:framework} with 
% UCB and exact matching machine.    
% The following theorem states a regret upper bound for $\mathcal{A}_1$.  

\begin{manualtheorem}{6}[Exact matching + UCB]
% Assumptions~\ref{asum:StableUnit:offline}, \ref{assumption:ignorability},
% \ref{asum:StableUnit:online} hold. 
Suppose there are $C$ possible categories of users' features $\bm{x}^1, \ldots, \bm{x}^C$.
Denote $\widehat{\MBP}[\bm{x}^c]$ as the fraction of online users whose context
is $\bm{x}^c$, whose expectation is $\MBP[\bm{x}^c]{\triangleq }\MBE[\widehat{\MBP}[\bm{x}^c]] $. 
Denote $a^\ast {\triangleq}
\arg\max_{\tilde{a}\in[K]}\MBE[y|\tilde{a}]$, $\Delta_a{\triangleq} \MBE[y|a^\ast]{-}\MBE[y|a]$.
Let $N(\bm{x}^c,a){\triangleq} \sum_{i\in[-I]}
\indicator{\bm{x}_i{=}\bm{x}^c,a_i{=}a}$ be the number of samples with context
$\bm{x}^c$ and action $a$.
Then,
% \vspace{-0.16in}
\begin{small}
\begin{align*}
  {R}(T, & \CA_0) \le \hspace{-0.04in}
\sum_{a\ne a^\ast} \left( 
1{+}\frac{\pi^2}{3} \hspace{-0.06in}  \right. \\
  + & \sum_{c\in[C]} \hspace{-0.03in} 
 \left.  \max\left\{0{,} 8\frac{\ln(T{+}A)}{\Delta_a^2}  
  \widehat{\MBP}[\bm{x}^c] {-} \hspace{-0.03in}
  \min_{\tilde{c}\in[C]} \hspace{-0.03in} \frac{ N(\bm{x}^{\tilde{c}}\hspace{-0.03in}{,}a)\MBP[\bm{x}^c]}{\MBP[\bm{x}^{\tilde{c}}]}\right\}  \right) \Delta_a,
\end{align*}
% \vspace{-0.08in}
\end{small}
  where the constant
\begin{small}
  \[
    A{=}N{-} \hspace{-0.05in}
    \sum_{a\ne a^\ast} \hspace{-0.03in}\sum_{c\in[C]} \hspace{-0.03in}
    \max \hspace{-0.03in} \left\{0,
      N(\bm{x}^{{c}}{,}a)   {-} (8\frac{\ln(T{+}N)}{\Delta_a^2}{+}1{+}\frac{\pi^2}{3}){\MBP}[\bm{x}^c]\right\}.
  \]
\end{small}
  \label{mthm:exact_matching}
\end{manualtheorem}
\vspace{-0.17in}
% the constant \min_{c\in[C]}N(\bm{x}^c,j) may be changed later

% {\color{blue} TODO: insights for the exact matching algorithm here}

\noindent
{
  Theorem~\ref{mthm:exact_matching} states how logged data reduces the regret.
  When there is no logged data, i.e. $N(\bm{x}_c,a)=0$, the regret bound
  $O(\log(T))$ is the same as that of UCB. 
}
If the number of logged data $N(\bm{x}^c,a)$ is greater
than $\widehat{\MBP}[\bm{x}^c]8{\ln(T+A)}/{\Delta_a^2} $ for each context
$\bm{x}^c$ and action $a$, then the regret is smaller than a constant.  
% In other words, when the amount of logged data is logarithmic w.r.t. the time $T$
% for each context $\bm{x}^c$ and action $a$, the decision maker
% has almost zero-regret by using the logged data.
In addition, when the 
regret $\Delta_a$ of choosing an action $a{\ne}a^\ast$ is smaller, we need more
logged data to make the regret close to zero.

% We point out that ``Historical UCB'' (HUCB) algorithm\cite{shivaswamy2012multi}
% is a special case of our algorithm $\CA_1$.
% Because HUCB ignores the context, we consider a dummy context $\bm{x}^1$. Then, we have
% $\widehat{\MBP}_a[\bm{x}^1]{=}1$ for $\forall
% a{\in}[K]$, and our regret bound is similar to that of HUCB.
% %  but our bound
% % has a smaller additional constant $1+\pi^2/3$.

One limitation of the exact matching evaluator is that 
when $\bm{x}$ is continous or has a high dimension, we can hardly find a sample in log-data with exactly the same context.   
% This may lead to a marginal improvement on the regret of the UCB algorithm.  
To address this limitation, we consider the 
propensity score matching method~\cite{stuart2010matching} $\CA_1$ in the main paper.
%  as an alternative to
% the exact matching method.
% \end{comment}

% \begin{comment}
\subsection{Inverse Propensity Score Weighting + UCB ($\CA_3$)}

% To further demonstrate the applicability of our framework, 
We now show how to use weighting methods~\cite{swaminathan2015counterfactual}\cite{kallus2018balanced} in causal inference.  

\noindent
{\bf Inverse propensity score (IPS) weighting. }
One can use the inverse of the propensity score $1/p$ as the weight. Then the estimated outcome $\bar{y}_a$ is a weighted average
from data (Line 4).
{
The intuition of IPS weighting is as follows: if an action is applied to users in group A more often
than users in other groups, then each sample for group A should have smaller 
weight so that the total weights of each group is proportional to
its population. In fact, the IPS weighting estimator is unbiased via {\em importance sampling}\cite{rubin2005causal}.
}
% \vspace{-0.15in}

Instance~\ref{alg:ipsw_match} shows the IPS weighting evaluator. We first estimate the
outcome $\bar{y}_a$ as the weighted average of logged outcomes.
Then, we calculate the {\em effective sample size} (a.k.a. ESS) $N_a$ of logged plays on the action $a$,
based on Hoeffding's inequalities~\cite{hoeffding1994probability}. 
After such initialization, the offline evaluator will return $\bar{y}_a$ w.r.t. action $a$ for $\lfloor {N_a} \rfloor$ times, and return NULL afterwards.

% \vspace{-0.1in}
\begin{algorithm}
 % \SetAlgorithmName{Class}{class}{List of Classes}
 \caption{\bf {\small (Offline Evaluator)} - IPS Weighting}\label{alg:ipsw_match}
 % \SetKwFunction{FInitISPW}{\bf initialize\_IPSW}
 % \Fn{\FInitISPW{}}{
 \begin{algorithmic}[1]
 \STATE {\bf Variables:} $\bar{y}_a,N_a (a{\in}[K])$ initialized by {\textbf{\_\_init\_\_($\CL$)}}
 % \SetKwFunction{FInit}{{\bf \_\_init\_\_}}
 \FUNCTION{\_\_init\_\_($\CL$)}
   \FOR{$a\in [K]$}
     \STATE $\bar{y}_a {\gets} \frac{\sum_{i\in[-I], a_i=a} y_i/p_i }{\sum_{i\in[-I],
         a_i=a} 1/p_i}$,~~~
     $N_a {\gets} \frac{ (\sum_{i\in[-I], a_i=a} 1/p_i)^2 }{ \sum_{i\in[-I], a_i=a} (1/p_i)^2 }$
   \ENDFOR
 \ENDFUNCTION
 % \SetKwFunction{FIPSW}{{\bf get\_outcome}}
 \FUNCTION{get\_outcome($\bm{x},a$)}
   \IF{$N_a\ge 1$}
     \STATE $N_a \gets N_a-1$
     \STATE \textbf{return} $\bar{y}_a$
   \ENDIF
   % \Else{
     \STATE \textbf{return} NULL
   % }
 \ENDFUNCTION
 \end{algorithmic}
\end{algorithm}
% \vspace{-0.2in}

\begin{manualtheorem}{7}[\bf IPS weighting + UCB]
% Suppose the propensity scores are correct.
% Assumptions~\ref{asum:StableUnit:offline}, \ref{assumption:ignorability}, \ref{asum:StableUnit:online} hold. 
 Suppose the online reward is bounded
$y_t\in[0,1]$ $\forall t{\in}[T]$ and the propensity score is bounded $p_i {\ge}
\bar{s} {>}0$ $\forall i\in[I]$, then the regret 
% \begin{small}
% \begin{align*}
$
R(T,\CA_3) \le
   \hspace{-0.05in}
  \sum_{a\ne a^\ast} \hspace{-0.03in}
  \Delta_a \hspace{-0.05in}
  \left( \max
  \left\{
    0, 8 \frac{\ln(T+\sum_{a=1}^K \lceil {N}_a \rceil)}{\Delta_a^2} {-}
    \lfloor{{N}_a} \rfloor
  \right\} {+} (1{+}\frac{\pi^2}{3})
  \right),
% \end{align*}
$
% \end{small}
where 
${N}_a {=}  {
    \left( \sum_{i\in [-I]} \frac{1}{p_i} \indicator{a_i{=}a} \right)^2
  }/{
     \sum_{i\in [-I]} \left( \frac{1}{p_i} \indicator{a_i{=}a}
      \right)^2 
  }
$.
%  and $n_j = \sum_{i\in[I]} \indicator{a_i=j}$ is the number of times action $j$
% is recorded in the logged data.
 \label{mthm:ipsw} 
 % \vspace{-0.15in}
\end{manualtheorem}

\noindent
Theorem \ref{mthm:ipsw} quantifies the impact of the logged data 
on the regret of the algorithm $\CA_3$.  
% The weighting method pre-processes the data to get the synthetic feedbacks
% for each action, 
Recall that ${N}_a$ is the
equivalent number of feedbacks for an action $a$.
When there is no logged data, i.e. ${N}_a=0$, the regret bound reduces
to the $O(\log{T})$ bound of UCB.
A larger
${N}_a$ indicates a lower regret bound (or a higher reduction of regret).
Notice that the number ${N}_a$ depends on the distribution of
logged data items' propensity scores. 
In particular, when all the propensity
scores are a constant $\tilde{p}$, i.e. $p_i{=}\tilde{p}$ $\forall i$, the effective
number is the actual number of plays of action $a$, i.e. 
$N_a{=}\sum_{i\in[-I]}\indicator{a_i=a}$.
When the
propensity scores $\{p_i\}_{i\in[-I]}$ have a more skewed distribution, the number ${N}_a$ will be smaller, leading to a larger
regret bound.  
% \end{comment}

\section{Case Study II: Contextual Decision}
\label{sec:sup_contextual}
% \begin{comment}
\subsection{Linear Regression + LinUCB ($\CA_4$) }
We consider that the outcomes follow a linear function:
\vspace{-0.1in}
\begin{align}
  y_t = \bm{\theta} \cdot \phi(\bm{x}_t, a_t) + \epsilon && \forall t\in[T],
  \label{eq:linear_form}
\vspace{-0.1in}
\end{align}
where $\phi(\bm{x},a)\in \mathbb{R}^m$ is an
$m$-dimensional {\em known} feature vector.  
The $\bm{\theta}$ is an $m$-dimensional {\em unknown} parameter to be learned, and $\epsilon$ is a random noise with $\mathbb{E}[\epsilon]{=}0$.
% The random noise $\epsilon$ comes from the unobserved confounders $\bm{u}$ in
% our model.
We instantiate our framework Algorithm~1 with ``LinUCB'' (Instance~\ref{alg:linUCB}) as the online bandit oracle
and ``linear regression'' (Instance~\ref{alg:linear_match}) as the offline
evaluator, to get an algorithm instance $\CA_4$.

\noindent{\bf LinUCB oracle.}
We use the LinUCB (Linear Upper Confidence Bound
algorithm~\cite{li2010contextual} in the following Instance~\ref{alg:linUCB} as the online learning oracle.  
The oracle estimates the unknown parameter
$\hat{\bm{\theta}}$ based on the feedbacks. The $\hat{y}_a{\triangleq} \hat{\bm{\theta}}^T
\phi(\bm{x},a) {+} \beta_t\sqrt{\phi(\bm{x},a)^T V^{-1} \phi(\bm{x},a)}$ is
the upper confidence bound of reward, where $\{\beta_t\}_{t=1}^T$ are
parameters. 
The oracle always plays the action
with the highest upper confidence bound.

  % \vspace{-0.1in}
\begin{algorithm}
  % \SetAlgorithmName{Class}{class}{List of Classes}
  \caption{\bf {\small (Online Bandit Oracle)} - LinUCB}\label{alg:linUCB}
  % \SetKwFunction{LinUCB}{{\bf LinUCB}}
  % {\bf Parameter:} $\alpha\in \MBR_+$\\
  \begin{algorithmic}[1]
  \STATE {\bf Variables:} a $d{\times}d$ matrix $V$ ($V{=}I_d$ intially),
  a $d$-dimentional vector $\bm{b}$ (initially $\bm{b}{=}\bm{0}$), initial time
  $t{=}1$ 
  
  \FUNCTION{play($\bm{x}$)}
    \STATE $\hat{\bm{\theta}} \gets V^{-1}\bm{b}$
    \FOR{$a\in [K]$}
      \STATE $\hat{y}_a \gets \hat{\bm{\theta}}^T \phi(\bm{\bm{x}, a}) +
      \beta_t \sqrt{\phi(\bm{x},a)^T V^{-1} \phi(\bm{x},a)}$
    \ENDFOR
    \STATE \textbf{return} $\arg\max_{a\in[K]} \hat{y}_a$
  \ENDFUNCTION
  \FUNCTION{update($\bm{x}, a, y$)}
    \STATE $V\gets V {+} \phi(\bm{x},a)\phi(\bm{x},a)^T$, \hspace{0.05in}
    $\bm{b} \gets \bm{b} {+} y\bm{x}$, \hspace{0.05in}
    $t\gets t{+}1$
  \ENDFUNCTION
  \end{algorithmic}
\end{algorithm}
  % \vspace{-0.1in}

\noindent{\bf Linear regression offline evaluator.}
 Instance~\ref{alg:linear_match} shows how we use linear regression to construct the offline evaluator.
From the logged data, we estimate the parameter $\hat{V}$ (Line 3), and the parameter $\hat{\bm{\theta}}$ (Line 4).
The offline evaluator always return the estimated outcome $\phi(\bm{x},a)\cdot
\hat{\bm{\theta}}$ by an linear model.
The offline evaluator will stop returning outcomes, 
when the logged data cannot
provide a tighter confidence bound than that of the online bandit oracle (Line 7
- 10).

% \vspace{-0.05in}
\begin{algorithm}
  % \SetAlgorithmName{Class}{class}{List of Classes}
  \caption{\bf {\small (Offline Evaluator)} - Linear Regression}\label{alg:linear_match}  \begin{algorithmic}[1]
  \STATE {\bf Variables:} $V, \hat{V}$ are $m{\times} m$ matrices,
  where $V$($\hat{V}$) is for the online/offline confidence bounds.
  $\hat{\bm{\theta}}$ is the estimated parameters. 
 $V$ is shared with LinUCB oracle.

  % \SetKwFunction{InitLin}{{\bf \_\_init\_\_}}
  \FUNCTION{\_\_init\_\_($\CL$)}
    \STATE $\hat{V}\gets \bm{I}_m + \sum_{i=1}^{N} \phi(\bm{x}_i,a_i) \cdot
    \phi(\bm{x}_i,a_i)^T$
\COMMENT{$\bm{I}_m$ is a $m\times m$ identity matrix}
    \STATE $\bm{b}\gets \sum_{i=1}^N y_i \cdot \phi(\bm{x}_i,a_i)$,
    $\hat{\bm{\theta}}\gets \hat{V}^{-1} \bm{b}$
  \ENDFUNCTION
  % \SetKwFunction{FLinear}{{\bf get\_outcome}}
  \FUNCTION{get\_outcome($\bm{x},a$)}
    \IF{$||\phi(\bm{x},a)||_{V+\phi(\bm{x}_i,a_i) \cdot
        \phi(\bm{x}_i,a_i)^T} > ||\phi(\bm{x},a)||_{\hat{V}}$}
      \STATE $V\gets V+\phi(\bm{x}_i,a_i) \cdot \phi(\bm{x}_i,a_i)^T$
      \STATE \textbf{return} $\phi(\bm{x},a) \cdot \hat{\bm{\theta}}$
    \ENDIF
    % \Else{
      \STATE \textbf{return} NULL
    % }
  \ENDFUNCTION
  \end{algorithmic}
\end{algorithm}
% \vspace{-0.15in}

%%% for journal use
% \begin{comment}
\begin{manualtheorem}{8}[Linear regr.+LinUCB, problem-independent]
Suppose we have $N$ offline data points. With probability at least $1-\delta$, the psuedo-regret 
\begin{align*}
& {R}(T,\CA_4) \le 
\sqrt{8 (N{+}T) \beta_T(\delta) \log \frac{ \texttt{trace}(V_0){+}(N{+}T)L^2
  }{\texttt{det} V_0 } }  \\
& -
 \sqrt{8\beta_T(\delta)} \min\{1, ||\bm{x}||_{\min}\} \frac{2}{L^2} \left( \sqrt{1+NL^2} - 1\right).
\end{align*}
Here, $\{\beta_{t}(\delta)\}_{t=1}^T$ is a non-decreasing sequence where
$\beta_t(\delta){\ge} 2d(1{+}2\ln(1/\delta))$, and $L{=}||\bm{x}||_{\max}$ is the
maximum of $l_2$-norm of the context in any time slot.  
\label{mthm:ContextDepend:LinPI}
\end{manualtheorem}

\noindent
The regret upper bound of Theorem \ref{mthm:ContextDepend:LinPI} consists of two parts. 
The first part from the online bandit oracle is $O(\sqrt{(N{+}T)\log(N{+}T)})$. The
second part is the reduction of regret by matching logged data which is $-\Omega(\sqrt{N\log(N+T)})$.
Comparing with the regret bound $O(\sqrt{T\log(T)})$ for only using the online feedbacks \cite{abbasi2011improved}, the regret bound
changes from $O(\sqrt{T\log(T)})$ to $O(\sqrt{(N+T)\log(N+T)}) -
\Omega(\sqrt{N\log(N+T)})$. For example, $\sqrt{N+T}{-}\sqrt{N}{=}\sqrt{T}\frac{\sqrt{T}}{\sqrt{N+T}+\sqrt{N}}{\le} \sqrt{T}$.

% {\color{blue} Li Ye: I am considering removing the problem-independent bound and
% only keep the problem-dependent bound}
% \end{comment}

We now show a regret bound for the problem-dependent case. 
Suppose in the specific problem, for any context $\bm{x}_t$, the difference of
expected rewards between the best and the {\em ``second best''} actions is at least $\Delta_{\min}$.
This is the settings of section 5.2 in the paper~\cite{abbasi2011improved}.

% \vspace{-0.05in}
\begin{manualtheorem}{9}[Linear regr.+LinUCB, problem dependent]
% Assumptions~\ref{asum:StableUnit:offline}, \ref{assumption:ignorability},
% \ref{asum:StableUnit:online} hold.
Suppose the rewards satisfy the linear model in Equation (\ref{eq:linear_form}).
Suppose offline evaluator returns a sequence $\{y_i\}_{i=1}^N$ w.r.t. $\{(\bm{x}_i,a_i)\}_{i=1}^N$. Let
$V_N {\triangleq} \sum_{i\in[N]} \bm{x}_i\bm{x}_i^T$,
$L{\triangleq}\max_{t{\le}T}\{||\bm{x}_t||_2\}$, and $\kappa {=} {TL^2}/{\lambda_{\min}(V_N)}$. Then 
\begin{align*}
{R}(T,\CA_4) \le
 \frac{8d(1+2\ln(T))}{\Delta_{\min}} d\log(1+\kappa) + 1.
\end{align*}
In particular, when the
smallest eigenvalue $\lambda_{\min}(V_N)\ge (1/2{+}\ln(T))T L^2$, the regret
is bounded by $16d^2/\Delta_{\min}{+}1$.
\label{mthm:linear_problem_dependent}
\end{manualtheorem}
\vspace{-0.15in}

{In Theorem~\ref{mthm:linear_problem_dependent} we see for a fixed
  $\kappa$, the regret is $\log(T)$ in $T$ time slots.}
Moreover, the above theorem highlights that when the logged data contains enough
information, so that $\lambda_{\min}(V_N)$ is greater than $(1/2+\ln(T))T$,
the regret can be upper bounded by a constant.

% \end{comment}
